# Supplementary material for: Minimal Presentation of $PSL(2,\mathbb{Z})$ Using Continuant Matrices with Integer Coefficients
Source: arXiv:2104.01274 source file (2021-04-02)
Supplement: Supplementary file 2 [file 99_AppendixB.tex]

\appendix
\chapter{Python Code to Calculate some Examples}
\label{app:B}
%\addcontentsline{toc}{chapter}{Appendix B}
In this appendix, the python code used to generate some of the examples in chapter 5 is presented. The core of the code is an algorithm performing a modification of the Euclidean algorithm to find the negative continued fraction expansion of the fraction $a/c$ where $a$ and $c$ are integers with gcd$(a,c)=1$. The core of this algorithm are functions named \textit{reducetwo}, \textit{reducethree} and \textit{reduceone}. The function \textit{reduce} is a combination of the three functions named in the last sentence. In the following, the code of this four functions is given:\\
\begin{em}
def reducetwo(R):\\
\hspace*{4mm}    i=1\\
\hspace*{4mm}    length=len(R)-1\\
\hspace*{4mm}    while i in range(length):\\
\hspace*{8mm}        if R[i]==2:\\
\hspace*{12mm}            count=1\\
\hspace*{12mm}            while R[i+count]==2:\\
\hspace*{16mm}                count=count+1\\
\hspace*{12mm}            if count>1:\\
\hspace*{16mm}                for k in range(count-1):\\
\hspace*{20mm}                    R=np.delete(R,[i+count-1-k])\\
\hspace*{12mm}                R[i-1]=R[i-1]-1\\
\hspace*{12mm}                R[i]=-count-1\\
\hspace*{12mm}                R[i+1]=R[i+1]-1\\
\hspace*{8mm}        i=i+1\\
\hspace*{8mm}        length=len(R)-1\\
\hspace*{4mm}    return(R)\\
def reducethree(R):\\
\hspace*{4mm}    i=1\\
\hspace*{4mm}    length=len(R)-1\\
\hspace*{4mm}    while i in range(length):\\
\hspace*{8mm}        if R[i]==2:\\
\hspace*{12mm}            count=1\\
\hspace*{12mm}            while R[i+count]==3:\\
\hspace*{16mm}                count=count+1\\
\hspace*{8mm}            if R[i+count]==2:\\
\hspace*{12mm}                for k in range(count):\\
\hspace*{16mm}                    R[i+k]=-3\\
\hspace*{12mm}                R[i-1]=R[i-1]-1\\
\hspace*{12mm}                R[i+count+1]=R[i+count+1]-1\\
\hspace*{12mm}                R=np.delete(R,[i+count])\\
\hspace*{8mm}        i=i+1\\
\hspace*{8mm}        length=len(R)-1\\
\hspace*{4mm}    return(R)\\
def reduceone(R):\\
\hspace*{4mm}    if len(R)>2:\\
\hspace*{8mm}        if R[len(R)-2]==1:\\
\hspace*{12mm}            R[len(R)-3]=R[len(R)-3]-1\\
\hspace*{12mm}            R[len(R)-1]=R[len(R)-1]-1\\
\hspace*{12mm}            R=np.delete(R,[len(R)-2])\\
\hspace*{8mm}        if R[len(R)-2]==-1:\\
\hspace*{12mm}            R[len(R)-3]=R[len(R)-3]+1\\
\hspace*{12mm}            R[len(R)-1]=R[len(R)-1]+1\\
\hspace*{12mm}            R=np.delete(R,[len(R)-2])\\
\hspace*{8mm}        if R[len(R)-2]==0:\\
\hspace*{12mm}            R[len(R)-3]=R[len(R)-3]+R[len(R)-1]\\
\hspace*{12mm}            R=np.delete(R,[len(R)-2,len(R)-1])\\
\hspace*{8mm}        if R[len(R)-2]==-2:\\
\hspace*{12mm}            R[len(R)-3]=R[len(R)-3]+1\\
\hspace*{12mm}            R[len(R)-1]=R[len(R)-1]+1\\
\hspace*{12mm}            R[len(R)-2]=2\\
\hspace*{4mm}    return(R)\\
def reduce(R):\\
\hspace*{4mm}    R=reducetwo(R)\\
\hspace*{4mm}    R=reducethree(R)\\
\hspace*{4mm}    if len(R)>2:\\
\hspace*{8mm}        while R[len(R)-2]<2 and R[len(R)-2]>-3:\\
\hspace*{12mm}            R=reduceone(R)\\
\hspace*{4mm}    return(R)\\
\end{em}
One wants to apply the function \textit{reduce} on a sequence $(c_1,...,c_n)$ corresponding to the presentation of a matrix $A \in PSL(2,\Z)$ as in lemma \ref{lm:unice} in order to obtain the unique minimal presentation of $A$ as in theorem \ref{sz:verylong}. First, the function \textit{reducetwo} eliminates all subsequences of consecutive twos from right to left using an operation of type (\ref{eqn:op2}) (except maybe at the beginning if $c_1=c_2=2$). There can be no error for too large indices since as long as we take a sequence of the form as in lemma \ref{lm:unice}, $c_n=0$, and hence, an appropriate end of the while-control flows is guaranteed.\\
The function \textit{reducethree} eliminates all subsequences of the form $(a,2,3,...,3,2,b)$ in an analogous matter and replaces them by subsequences $(a-1,-3,...,-3,b-1)$ that are by one entry shorter and represent the same matrix (see also lemma \ref{lm:232}). Note that this may produce new subsequences of consecutive twos. But those have at most length two (since the function \textit{reducetwo} was already performed before), and since the function strictly works from left to right, they occur only at the right of the subsequence replaced in the last step. Hence, the function will recognize a newly created subsequence of the form $(a,2,2,b)$ as a subsequence of the form $(a,2,3,...,3,2,b)$ where the number of threes is zero, and so it will transform the subsequence into $(a-1,-3,b-1)$ what would also be the outcome if applying an operation of type (\ref{eqn:op2}) with $k=2$. This becomes more clear in example \ref{bsp:232}.\\
The function reduceone eliminates the entry second to last if it contradicts minimality or transforms it into a two if it was -2 before.\\
The first two operations do not create entries in $\{-2,-1,0,1\}$ except maybe at the beginning or at the end of the sequence if one starts with a sequence as in lemma \ref{lm:unice}. The same holds for operation \textit{reduceone} if the replaced entry is -2, -1 or 0. If this entry is one, the sequence may end on $(a,2,1,0)$, and then operation \textit{reduceone} transforms the end into $a,1,-1$, but since the operation is repeated until the second last entry is not in $\{-2,-1,0,1\}$ (or the length of the sequence smaller than three) and operation \textit{reduceone} does never generate such entries except at the two last positions, at the end, the resulting sequence will be minimal and not contain any -2's, i.e. it will be the unique sequence related to $A$ as in theorem \ref{sz:verylong}.\\
Now, one may apply the following code:\\
\begin{em}
length = eval(input("length: "))\\
S = np.array([])\\
for i in range (length):\\
\hspace*{4mm}    S = np.append(S,eval(input("Zahl: ")))\\
G=np.eye(2)\\
for i in range(len(S)):\\
\hspace*{4mm}    A=np.array([[S[i],-1],[1,0]])\\
\hspace*{4mm}    G=np.matmul(G,A)\\
if G[1,0] < 0:\\
\hspace*{4mm}    G=-G\\
print(G)\\
x=G[0,0]\\
y=G[1,0]\\
z=G[1,1]\\
w=G[0,1]\\
Q = np.array([])\\
if y>0:\\
\hspace*{4mm}    m=math.ceil(z/y)\\
\hspace*{4mm}    while y > 0:\\
\hspace*{8mm}        q=math.ceil(x/y)\\
\hspace*{8mm}        platzhalter=y\\
\hspace*{8mm}        y=q*y-x\\
\hspace*{8mm}        x=platzhalter\\
\hspace*{8mm}        Q = np.append(Q,q)\\
else:\\
\hspace*{4mm}    m=w/x\\
Q = np.append(Q,m)\\
Q = np.append(Q,0)\\
print(Q)\\
R=reduce(Q)\\
print(R)\\
\end{em}
The script takes an arbitrary sequence of integers as input. First, one has to specify the length of the sequence, and then, one has to enter the entries of the sequence $(c_1,...,c_n)$. The script returns the continuant matrix $M(c_1,...,c_n)$ (normalized by a factor of -1 if the lower left entry is initially negative), its unique presentation $Q$ as in lemma \ref{lm:unice} and its unique minimal presentation $R$ as in theorem \ref{sz:verylong}. The while-control flow performs the modified Euclidean algorithm to find out the negative continued fraction expansion of $a/c$ where $a$ is the upper left entry and $c$ the lower left entry of the matrix.\\
Slightly modified, the script looks like this:\\
\begin{em}
a = eval(input("a: "))\\
b = eval(input("b: "))\\
c = eval(input("c: "))\\
d = eval(input("d: "))\\
G=np.array([[a,b],[c,d]])\\
if G[1,0] < 0:\\
\hspace*{4mm}    G=-G\\
print(G)\\
x=G[0,0]\\
y=G[1,0]\\
z=G[1,1]\\
w=G[0,1]\\
Q = np.array([])\\
if y>0:\\
\hspace*{4mm}    m=math.ceil(z/y)\\
\hspace*{4mm}    while y > 0:\\
\hspace*{8mm}        q=math.ceil(x/y)\\
\hspace*{8mm}        platzhalter=y\\
\hspace*{8mm}        y=q*y-x\\
\hspace*{8mm}        x=platzhalter\\
\hspace*{8mm}        Q = np.append(Q,q)\\
else:\\
\hspace*{4mm}    m=w/x\\
Q = np.append(Q,m)\\
Q = np.append(Q,0)\\
print(Q)\\
R=reduce(Q)\\
print(R)\\
\end{em}
Here, one enters not a sequence but directly the four entries $a,b,c$ and $d$ of a matrix$A=\begin{pmatrix}a&b\\c&d\end{pmatrix}$  in $PSL(2,\Z)$. The script again returns the matrix itself (multiplied by -1 if $c<0$), its unique presentation $Q$ as in lemma \ref{lm:unice} and its unique minimal presentation $R$ as in theorem \ref{sz:verylong}. Note that the script allows also to enter a matrix that has a determinant not equal to one. In this case, the script will still provide a result, but this result will be something arbitrary.

\begin{bsp}
Consider the sequence $(5,2,3,3,2,3,2,5)$. Then, the function \textit{reducethree} will first transform it into $(4,-3,-3,-3,2,2,5)$. Now, there is a new subsequence of two consecutive twos. But the function \textit{reducethree} will interpret the subsequence $(-3,2,2,5)$ as a subsequence of the form $(a,2,3,...,3,2,b)$ with $a=-3$ and $b=5$ where the number of threes is zero. Hence, it will be transformed into $(-4,-3,4)$, and as the result of the reduction process of the whole sequence, one gets $(4,-3,-3,-4,-3,4)$.
\label{bsp:232}
\end{bsp}
